# Supplementary material for: Trickery: Exploring a Serious Game Approach to Raise Awareness of Deceptive Patterns
Source: arXiv:2401.06247 source file (2024-10-24)
Supplement: Supplementary file 1 [file appendix.tex]

\newpage
\appendix
\section{Appendix A: Detailed Definitions of Educational Dark Pattern Analogies}
\label{appendix}
To present the educational dark pattern analogies, we have adapted the privacy dark pattern framework by \citeauthor{Bosch.2016} \cite{Bosch.2016}. While this framework is specifically used for privacy dark patterns, we believe that its structure is equally applicable to educational dark pattern analogies, as it provides a structure that allows us to contextualize dark pattern concepts with the corresponding educational dark pattern analogies. Through the \emph{Strategies} and \emph{Related Patterns} fields of the framework, designers may find inspiration in educational dark pattern analogies that do not specifically match the dark pattern concept they want to convey and adapt them to their needs. To differentiate between the educational dark pattern analogies and the dark pattern concepts they adapt, we introduce the \emph{Dark Pattern Concept} field and give the educational dark pattern analogies their own unique names. As our specific implementations only represent one possible way to implement the educational dark pattern analogies, we describe the educational dark pattern analogy in \emph{Description}, and our specific implementation in \emph{Examples / Known Uses}. 

\vspace{12pt}
\tablefirsthead{}
\tablehead{\hline \multicolumn{2}{|r|} {Continued from previous page} \\ \hline}
\tabletail{\hline \multicolumn{2}{|r|} {Continued on next page} \\ \hline}
\tablelasttail{}

\begin{xtabular}{|l|l|}
        \hline
        \multicolumn{2}{|c|}{\textbf{Insensible Key Mapping}} \\
        
        \hline
        \textbf{Dark Pattern Concept:} & Preselection \cite{Gray.26.04.2018} \\
        \hline
        \textbf{Strategies:} & FAKE, OBSCURE, VIOLATE \\
        \hline
        \textbf{Related Patterns:} & Sneaking, Aesthetic Manipulation \\
        \hline
        \multicolumn{2}{|l|}{\textbf{Description:}} \\
        \multicolumn{2}{|p{\dimexpr\linewidth-2\tabcolsep}|}
        {The analogy claims to provide the players with a helpful control keyboard mapping. In truth, the keyboard mapping is designed to inhibit the players’ movement.} \\
        \hline
        \multicolumn{2}{|l|}{\textbf{Examples / Known Uses:}} \\
        \multicolumn{2}{|p{\dimexpr\linewidth-2\tabcolsep}|}
        {The narrator in our game asks the player to accept a "fine-tuned control specially chosen for you". However, the key mapping of this control maps the player's movement to keys spread far from each other, inhibiting ease of play.} \\
        \hline
        \multicolumn{2}{|l|}{\textbf{Context:}} \\
        \multicolumn{2}{|p{\dimexpr\linewidth-2\tabcolsep}|}
        {Website providers often preselect values that disclose more personal user information to them than is necessary for the website to function (e.g., cookie consent banners having consent for Third-Party-Cookies preselected). The consequences of this data collection are usually not immediately noticeable to the users.} \\
        \hline
        \multicolumn{2}{|l|}{\textbf{Effect:}} \\
        \multicolumn{2}{|p{\dimexpr\linewidth-2\tabcolsep}|}
        {Players trying to play the game with the preselected key mapping should quickly notice that accepting the preselection without thinking about it inhibits their ability to play the game. Unlike in real examples of Preselection, the negative consequences of accepting the Preselection are immediately noticeable.} \\
        \hline
        \multicolumn{2}{|l|}{\textbf{Countermeasures:}} \\
        \multicolumn{2}{|p{\dimexpr\linewidth-2\tabcolsep}|}
        {Players can change the key mapping to a more usable one designed by following common key mappings for the game genre (e.g., using WASD for movement in a PC first-person game or clicking on a target location in point-and-click adventures). In subsequent playthroughs, players can choose to decline the offer to use the preselected key mapping. However, as with real examples of the preselection dark pattern, they should still have to select their key mapping in the menu, similar to many Cookie Consent Banners hiding their preferences behind a “Change Settings” button.} \\
        \hline
        \multicolumn{2}{|l|}{\textbf{Psychological Aspects:}} \\
        \multicolumn{2}{|p{\dimexpr\linewidth-2\tabcolsep}|}
        {At the start of the game, we assume the users have a certain amount of trust in the game and would like to get going quickly. Many games have a tutorial stage, so players might assume this is part of a tutorial. Therefore, System 1 thinking is prompted and players might not think twice about accepting the preselected key mapping. This is akin to users wanting to get to a website’s contents quickly, accepting all cookies. Unlike real examples of Preselection, this scenario triggers System 2 thinking with an immediate negative consequence: a very unusual game experience.} \\
        \hline
        \multicolumn{2}{|c|}{\vspace{-7pt}}\\
        \multicolumn{2}{|c|}{\includegraphics[width=\dimexpr\linewidth-2\tabcolsep]{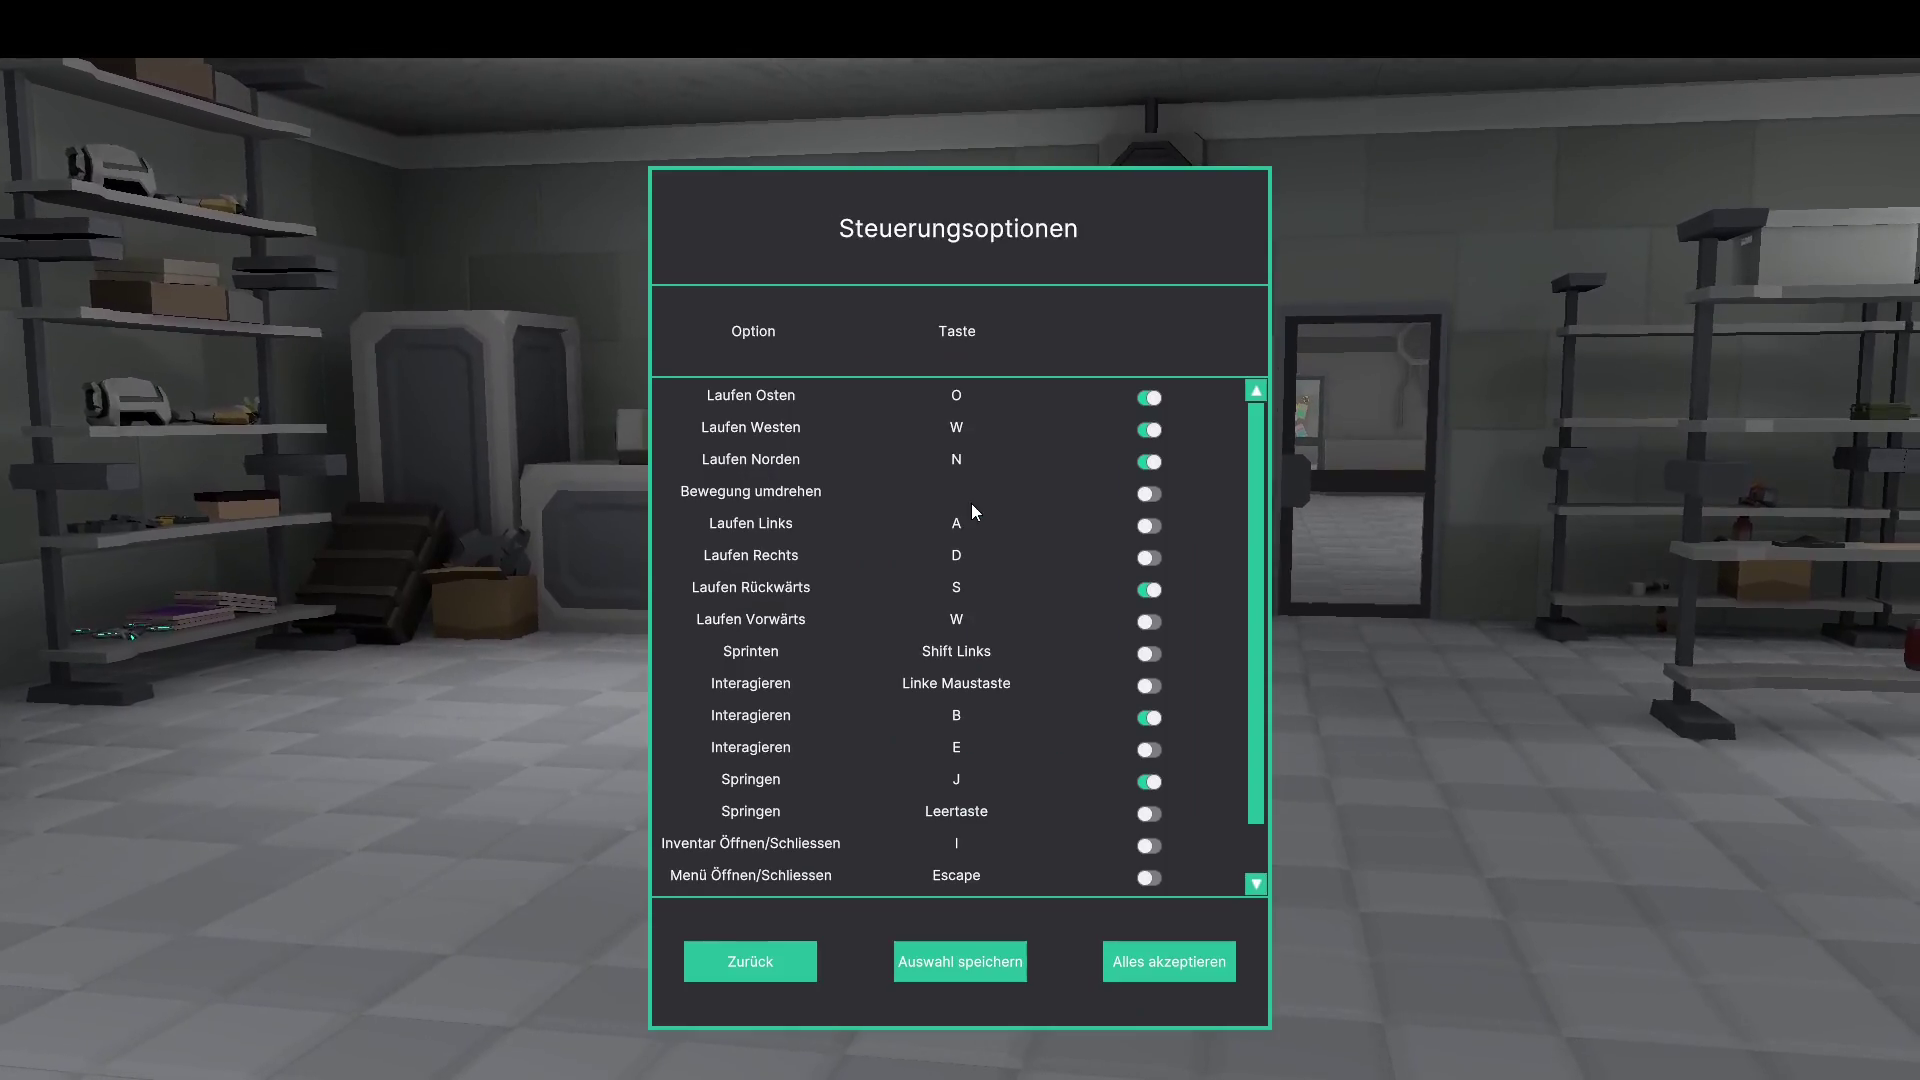}} \\
        \multicolumn{2}{|p{\dimexpr\linewidth-2\tabcolsep}|}{\small \textbf{Figure 4:} Insensible Key Mapping represented in the control menu of our game.}\\
        \hline
\end{xtabular}
\vspace{5cm}

\tablefirsthead{}
\tablehead{\hline \multicolumn{2}{|r|} {Continued from previous page} \\ \hline}
\tabletail{\hline \multicolumn{2}{|r|} {Continued on next page} \\ \hline}
\tablelasttail{}

\begin{xtabular}{|l|l|}
        \hline
        \multicolumn{2}{|c|}{\textbf{Sneaky Shop}} \\
        \hline
        \textbf{Dark Pattern Concept:} & Sneaking \cite{Gray.26.04.2018} \\
        \hline
        \textbf{Strategies:} & MAXIMIZE, OBSCURE \\
        \hline
        \textbf{Related Patterns:} & Preselection, Hidden Information \\
        \hline
        \multicolumn{2}{|l|}{\textbf{Description:}} \\
        \multicolumn{2}{|p{\dimexpr\linewidth-2\tabcolsep}|}
        {The analogy tasks players with buying a list of items from a shop. The analogy claims the shop provides the players with what they need, adding additional items to the checkout without explicit notification. The analogy then checks which items were bought and discards the entire batch if the bought items do not match the list.} \\
        \hline
        \multicolumn{2}{|l|}{\textbf{Examples / Known Uses:}} \\
        \multicolumn{2}{|p{\dimexpr\linewidth-2\tabcolsep}|}
        {The players in our game have to buy equipment from an AI-powered vending machine for their new job. The vending machine adds supposedly helpful items to the shopping cart. A disinfection machine checks whether the items match the required equipment and recycles the bought equipment if it does not.} \\
        \hline
        \multicolumn{2}{|l|}{\textbf{Context:}} \\
        \multicolumn{2}{|p{\dimexpr\linewidth-2\tabcolsep}|}
        {Websites may try to use sneaking to gain consent for subscriptions or to sell users unnecessary items, e.g. by having a default option be the subscription and users having to manually select the one-time purchase. A similar example of sneaking employed by websites is putting the optional checkbox for a newsletter subscription right below the required checkbox for terms and conditions, leading users to believe that a newsletter subscription is required.} \\
        \hline
        \multicolumn{2}{|l|}{\textbf{Effect:}} \\
        \multicolumn{2}{|p{\dimexpr\linewidth-2\tabcolsep}|}
        {Players who do not notice the items snuck into their checkout immediately get rejected when the game checks for the matching list. This causes them to rethink what might have caused the rejection and look at the items they selected and the checkout screen more carefully.} \\
        \hline
        \multicolumn{2}{|l|}{\textbf{Countermeasures:}} \\
        \multicolumn{2}{|p{\dimexpr\linewidth-2\tabcolsep}|}
        {Players cannot prevent the sneaking from happening, but they can be vigilant before completing the purchase. Like in real examples of Sneaking, they are able to de-select the additional items before completing the purchase} \\
        \hline
        \multicolumn{2}{|l|}{\textbf{Psychological Aspects:}} \\
        \multicolumn{2}{|p{\dimexpr\linewidth-2\tabcolsep}|}
        {As there is no notification of additional items being added, players would assume that they do not need to critically think about their purchases and just pick the necessary items from the list. A mistake is immediately made clear by the game upon finishing the purchase. Discarding the entire cart forces the players to redo the shopping. Unlike in real life, where such a purchase is likely to be noticed only once the goods arrive or additional costs are billed, the consequences of not checking the purchase properly are immediately made clear to the players, engaging System 2 thinking in the next attempted purchase.} \\
        %\hline
        \multicolumn{2}{|c|}{\vspace{-7pt}}\\
        \multicolumn{2}{|c|}{\includegraphics[width=\dimexpr\linewidth-2\tabcolsep]{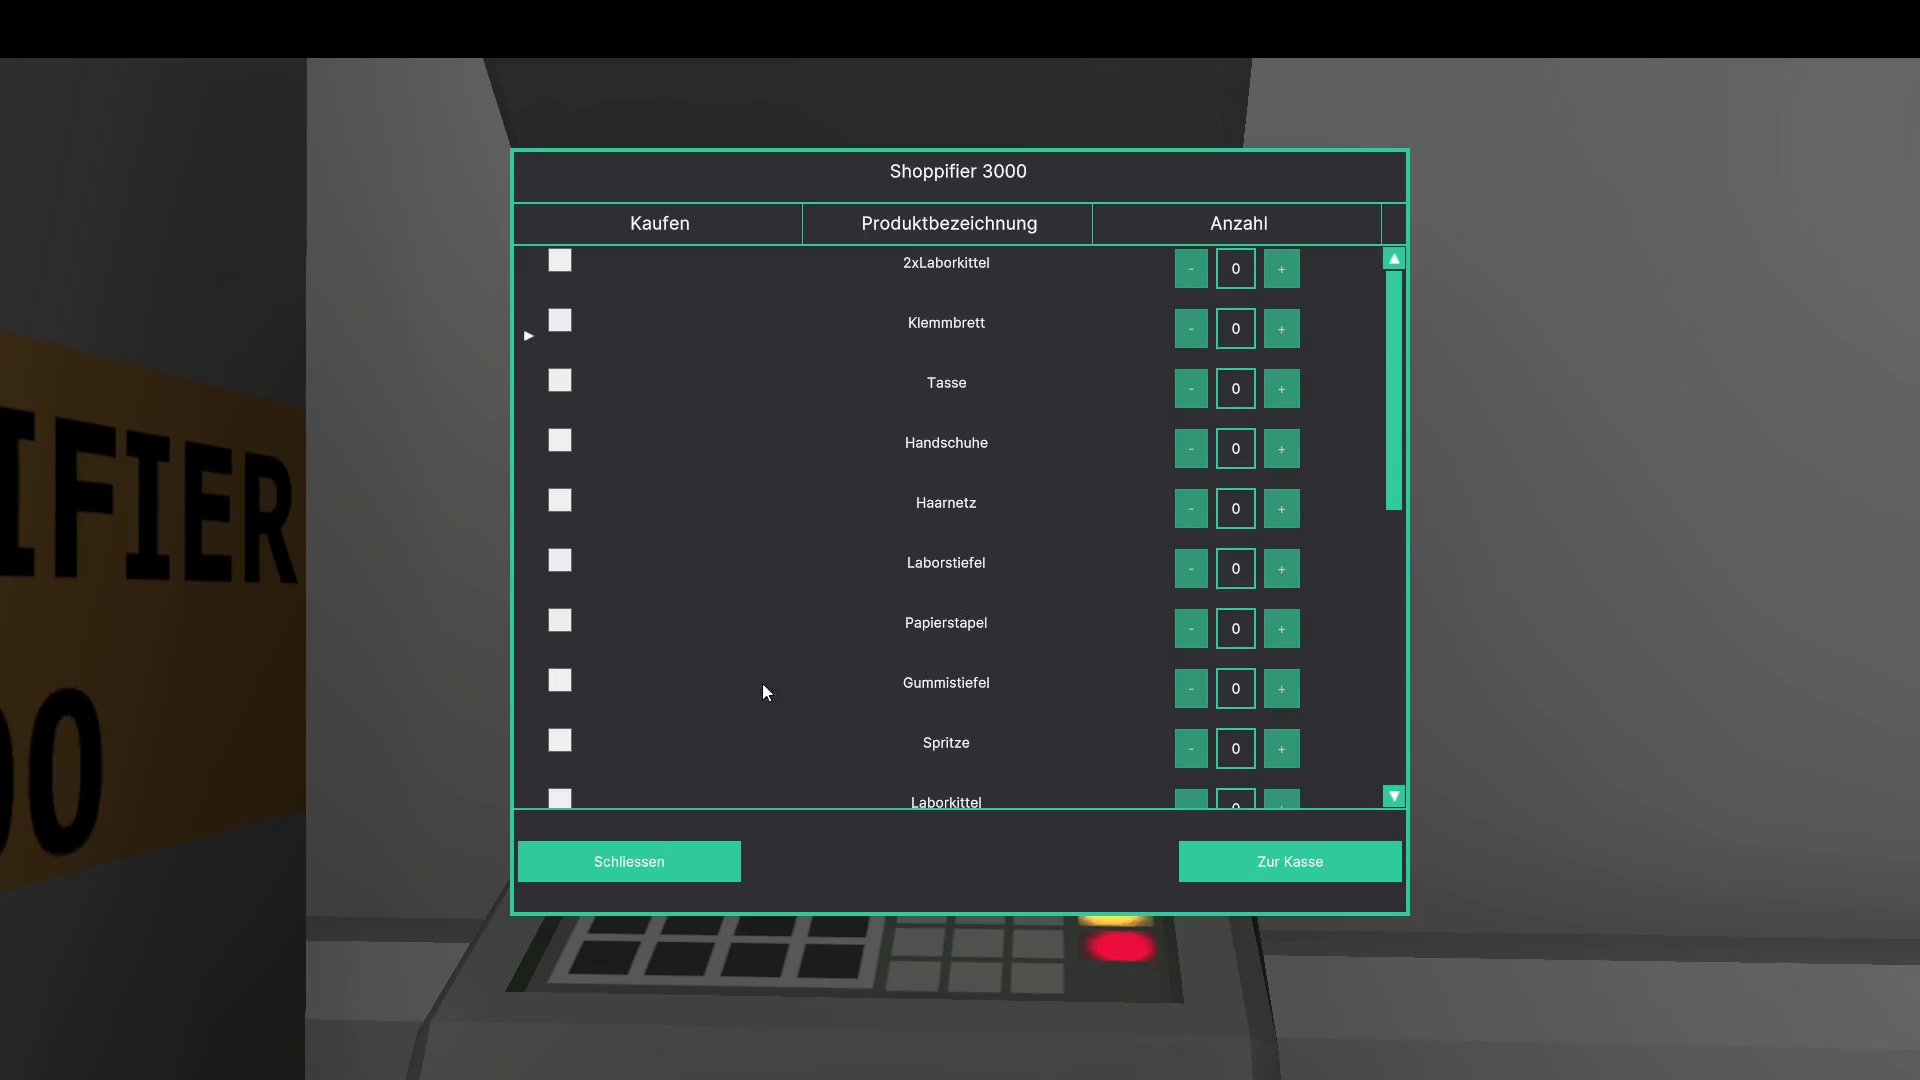}} \\
        \multicolumn{2}{|p{\dimexpr\linewidth-2\tabcolsep}|}{\small \textbf{Figure 5:} Sneaky Shop represented as a graphical user interface in our game.}\\
        \hline
\end{xtabular}
\vspace{50pt}

\tablefirsthead{}
\tablehead{\hline \multicolumn{2}{|r|} {Continued from previous page} \\ \hline}

\tabletail{\hline \multicolumn{2}{|r|} {Continued on next page} \\ \hline}
\tablelasttail{}

\begin{xtabular}{|l|p{\dimexpr\linewidth/2}|}
        \hline
        \multicolumn{2}{|c|}{\textbf{Walls of Text}} \\*
        \hline
        \textbf{Dark Pattern Concept:} & Hidden Information \cite{Gray.26.04.2018} \\*
        \hline
        \textbf{Strategies:} & MAXIMIZE, OBSCURE \\*
        \hline
        \textbf{Related Patterns:} & Sneaking, Aesthetic Manipulation, Obstruction \\*
        \hline
        \multicolumn{2}{|l|}{\textbf{Description:}} \\
        \multicolumn{2}{|p{\dimexpr\linewidth-2\tabcolsep}|}
        {The analogy presents multiple long texts to the players. To proceed, they must carefully read the texts to discover hidden clues to riddles or puzzles. Solving the puzzles allows them to proceed.} \\
        \hline
         \multicolumn{2}{|l|}{\textbf{Examples / Known Uses:}} \\
        \multicolumn{2}{|p{\dimexpr\linewidth-2\tabcolsep}|}
        {The players in our game walk into a room with four screens, each showing a text about the rules of the laboratory. To show that they have read the texts carefully, eight levers on the ground need to be put in the correct combination to unlock the door. Players can discover the combination by finding the hidden key to press for each screen and solving the riddle/puzzle hidden behind the screen using the hints provided in the text.} \\
        \hline
        \multicolumn{2}{|l|}{\textbf{Context:}} \\
        \multicolumn{2}{|p{\dimexpr\linewidth-2\tabcolsep}|}
        {Privacy policies, as well as terms and conditions, need to be accepted when using a service. These policies contain information about how personal data is handled by the website providers, including which third parties may gain access to the data. Oftentimes, users do not read these policies due to their length and language, instead opting to just accept the privacy policy to quickly gain access to the service \cite{Bosch.2016}. Similarly, websites may hide relevant options behind collapsable elements, such as opt-out options \cite{Gray.26.04.2018}} \\
        \hline
        \multicolumn{2}{|l|}{\textbf{Effect:}} \\
        \multicolumn{2}{|p{\dimexpr\linewidth-2\tabcolsep}|}
        {Players are overwhelmed by the amount of text they are supposed to read, leading to frustration. Players may try to find a less involved solution, such as searching for an alternative path or only skimming the text. As the game provides no other options or hints to solve the riddles, players will inevitably have to read the texts.} \\
        \hline
        \multicolumn{2}{|l|}{\textbf{Countermeasures:}} \\
        \multicolumn{2}{|p{\dimexpr\linewidth-2\tabcolsep}|}
        {Unlike in real examples of Hidden Information, where users can choose to not look for the information and instead just continue using the website, players must read the entire text to progress.} \\
        \hline
        \multicolumn{2}{|l|}{\textbf{Psychological Aspects:}} \\
        \multicolumn{2}{|p{\dimexpr\linewidth-2\tabcolsep}|}
        {Understanding complex and long texts requires System 2 thinking. When websites hide information in long text and still allow users to use the website, System 1 thinking takes over and prevents users from searching for and discovering information that may lead them to refrain from using the service. This Educational Dark Pattern Analogy does not offer users a viable alternative to reading the texts. Players may at first try to find a solution that falls outside the scope of the scenario, but will eventually have to engage in System 2 thinking and read the texts to proceed to the next scenario. The frustration experienced in recognizing that the only sensible option is to read the texts is supposed to stick with users and remind them of the negative consequences they may encounter in real examples of Hidden Information.} \\
        %\hline
        \multicolumn{2}{|c|}{\vspace{-7pt}}\\
        \multicolumn{2}{|c|}{\includegraphics[width=\dimexpr\linewidth-2\tabcolsep]{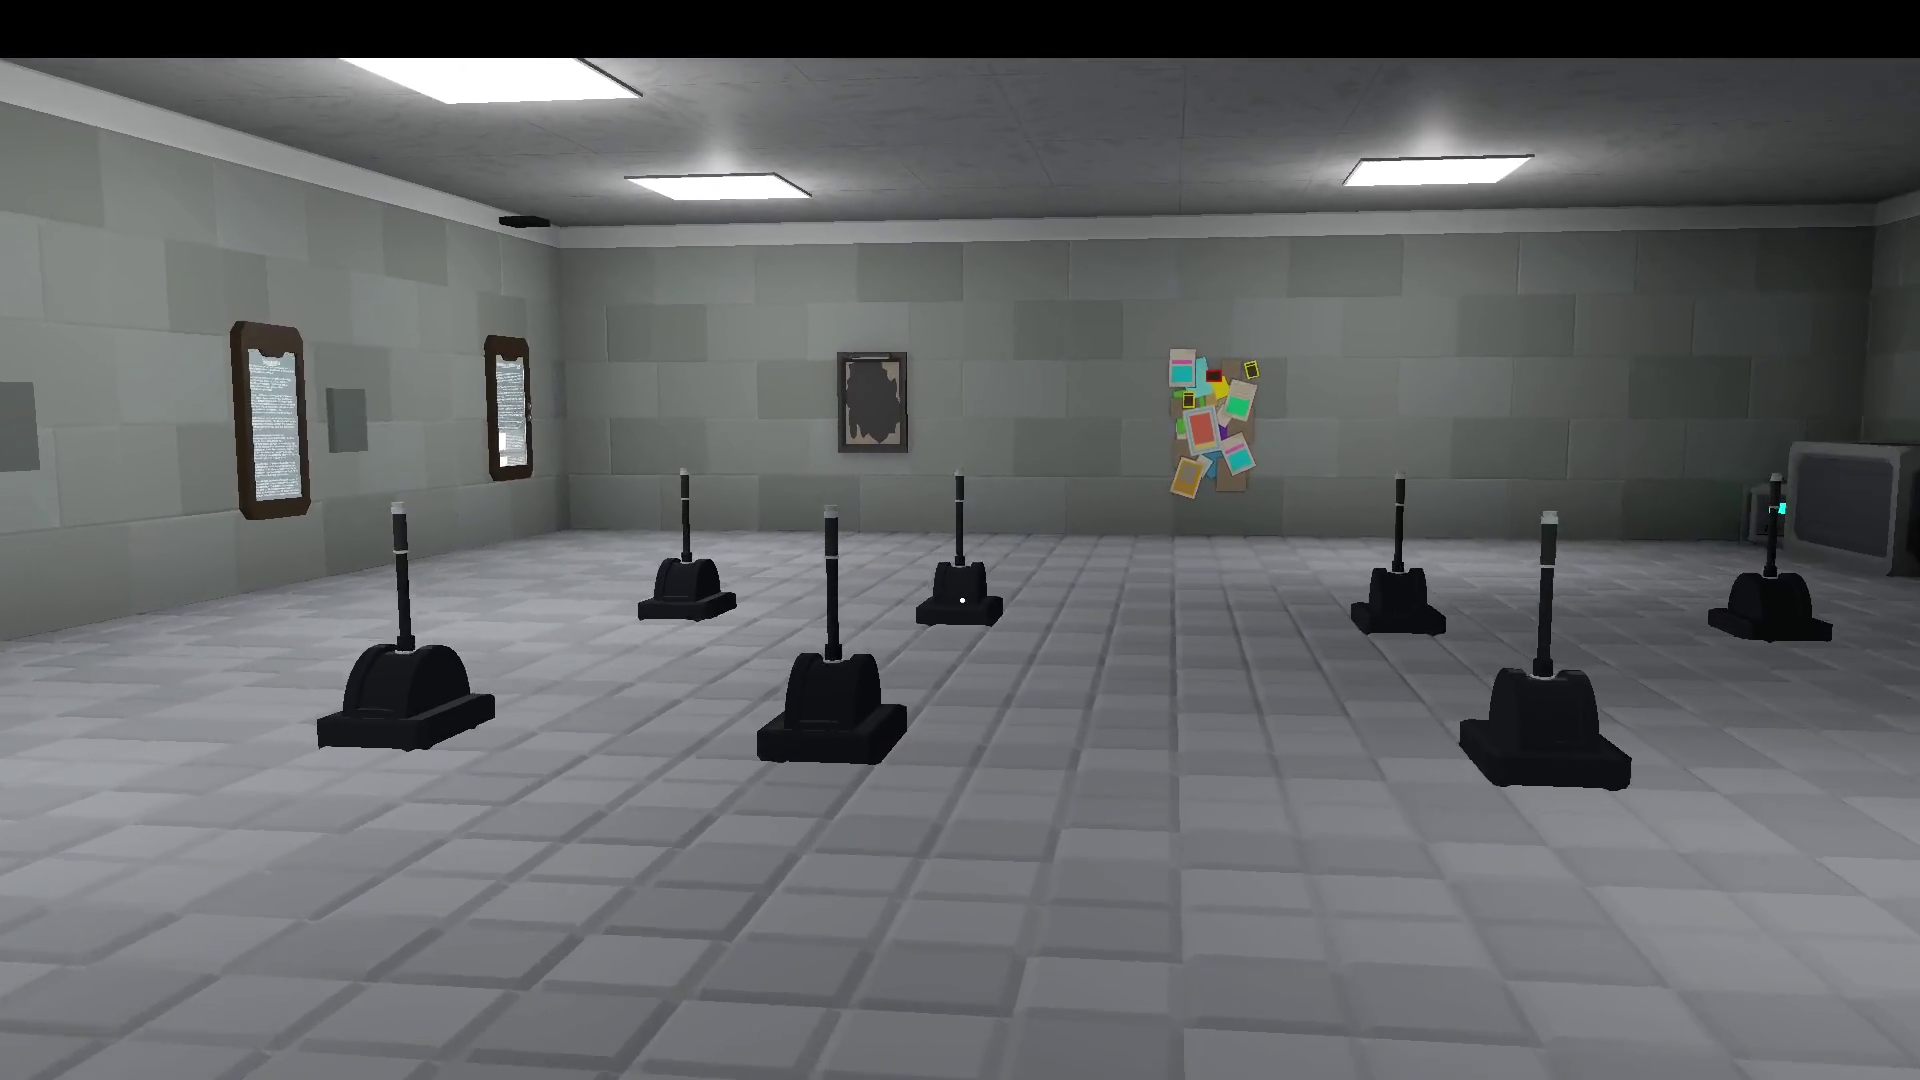}} \\
        \multicolumn{2}{|p{\dimexpr\linewidth-2\tabcolsep}|}{\small \textbf{Figure 6:} Walls of Text represented as screens on the left wall in our game.}\\
        \hline
\end{xtabular}
\vspace{12pt}

\tablefirsthead{}
\tablehead{\hline \multicolumn{2}{|r|} {Continued from previous page} \\ \hline}

\tabletail{\hline \multicolumn{2}{|r|} {Continued on next page} \\ \hline}
\tablelasttail{}

\begin{xtabular}{|l|l|}
        \hline
        \multicolumn{2}{|c|}{\textbf{Winding Hallway \& Shortcut}} \\
        \hline
        \textbf{Dark Pattern Concept:} & Aesthetic Manipulation \cite{Gray.26.04.2018} \\
        \hline
        \textbf{Strategies:} & OBSCURE \\
        \hline
        \textbf{Related Patterns:} & Hidden Information \\
        \hline
        \multicolumn{2}{|l|}{\textbf{Description:}} \\
        \multicolumn{2}{|p{\dimexpr\linewidth-2\tabcolsep}|}
        {The analogy provides the players with a wide and long room illuminated only in the middle. The edges of the room are dark. The players' goal is to move towards the end of the room, with the illuminated path being the most obvious choice. The illuminated path however leads to a winding hallway that significantly increases the duration of the journey. The players may explore the dark areas of the room and find a shortcut to the next room that goes in a straight line from the start of the shortcut to the end of the winding hallway. The analogy needs to make players aware of a possible shortcut through some sort of cue. The exits of both the hallway and the shortcut are at the same place. \vspace{6pt}} \\
        \hline
        \multicolumn{2}{|l|}{\textbf{Examples / Known Uses:}} \\
        \multicolumn{2}{|p{\dimexpr\linewidth-2\tabcolsep}|}
        {In our game, players enter a large room illuminated only in the middle by spotlights. The narrator instructs them to follow the illuminated path. At the end of the path, a break room is visible, however, the players cannot enter it. Instead, to the right of the break room, there is an entrance to the winding hallway, which is fully illuminated. The walls of the hallway are plastered with advertisements. If players search the dark areas of the large room, players may find a hidden door, disguised as a wall under a broken lamp, leading to a dark corridor that can be used as a shortcut to avoid the winding hallway.} \\
        \hline
        \multicolumn{2}{|l|}{\textbf{Context:}} \\
        \multicolumn{2}{|p{\dimexpr\linewidth-2\tabcolsep}|}
        {Websites often present a choice between two or more options with a false hierarchy by manipulating the aesthetic of the interface elements. A popular example is using a colored button for one option while only using text for the other. Another example is requiring more clicks for one option than another. This causes users to gravitate towards using the more appealing option, which is often the option where more information about the user is disclosed.} \\
        \hline
        \multicolumn{2}{|l|}{\textbf{Effect:}} \\
        \multicolumn{2}{|p{\dimexpr\linewidth-2\tabcolsep}|}
        {The illuminated part of the room and the break room at the end which seems to be the next part of the game represents the option the website providers would want users to take. The dark parts of the room, which players can explore but are discouraged from doing so by the aesthetic, represent the more privacy-preserving option. The light seems more inviting, but following its path leads to an unpleasant consequence, the long hallway with advertisements.} \\
        \hline
        \multicolumn{2}{|l|}{\textbf{Countermeasures:}} \\
        \multicolumn{2}{|p{\dimexpr\linewidth-2\tabcolsep}|}
        { Players should ignore the appealing illuminated path and explore the dark areas of the room. This way, they will skip over the long and winding hallway, finishing this part of the game much quicker. This is similar to using the less prominent, but more privacy-preserving option when faced with a real example of Aesthetic Manipulation.} \\
        \hline
        \multicolumn{2}{|l|}{\textbf{Psychological Aspects:}} \\
        \multicolumn{2}{|p{\dimexpr\linewidth-2\tabcolsep}|}
        {The scenario prompts System 1 thinking, by leading players to follow the visually appealing illuminated path. Unlike in real examples of Aesthetic Manipulation, where the alternative path is deliberately obscured, a cue for the shortcut prompts System 2 thinking, encouraging exploration of alternative options. Players who follow the illuminated path face the consequence of having to walk through the winding hallway. Placing the end of the shortcut and the winding hallway at the same place prompts users who follow the winding hallway to recognize that they could have taken a shorter path.} \\
        \hline
        \multicolumn{2}{|c|}{\vspace{-7pt}}\\
        \multicolumn{2}{|c|}{\includegraphics[width=\dimexpr\linewidth-2\tabcolsep]{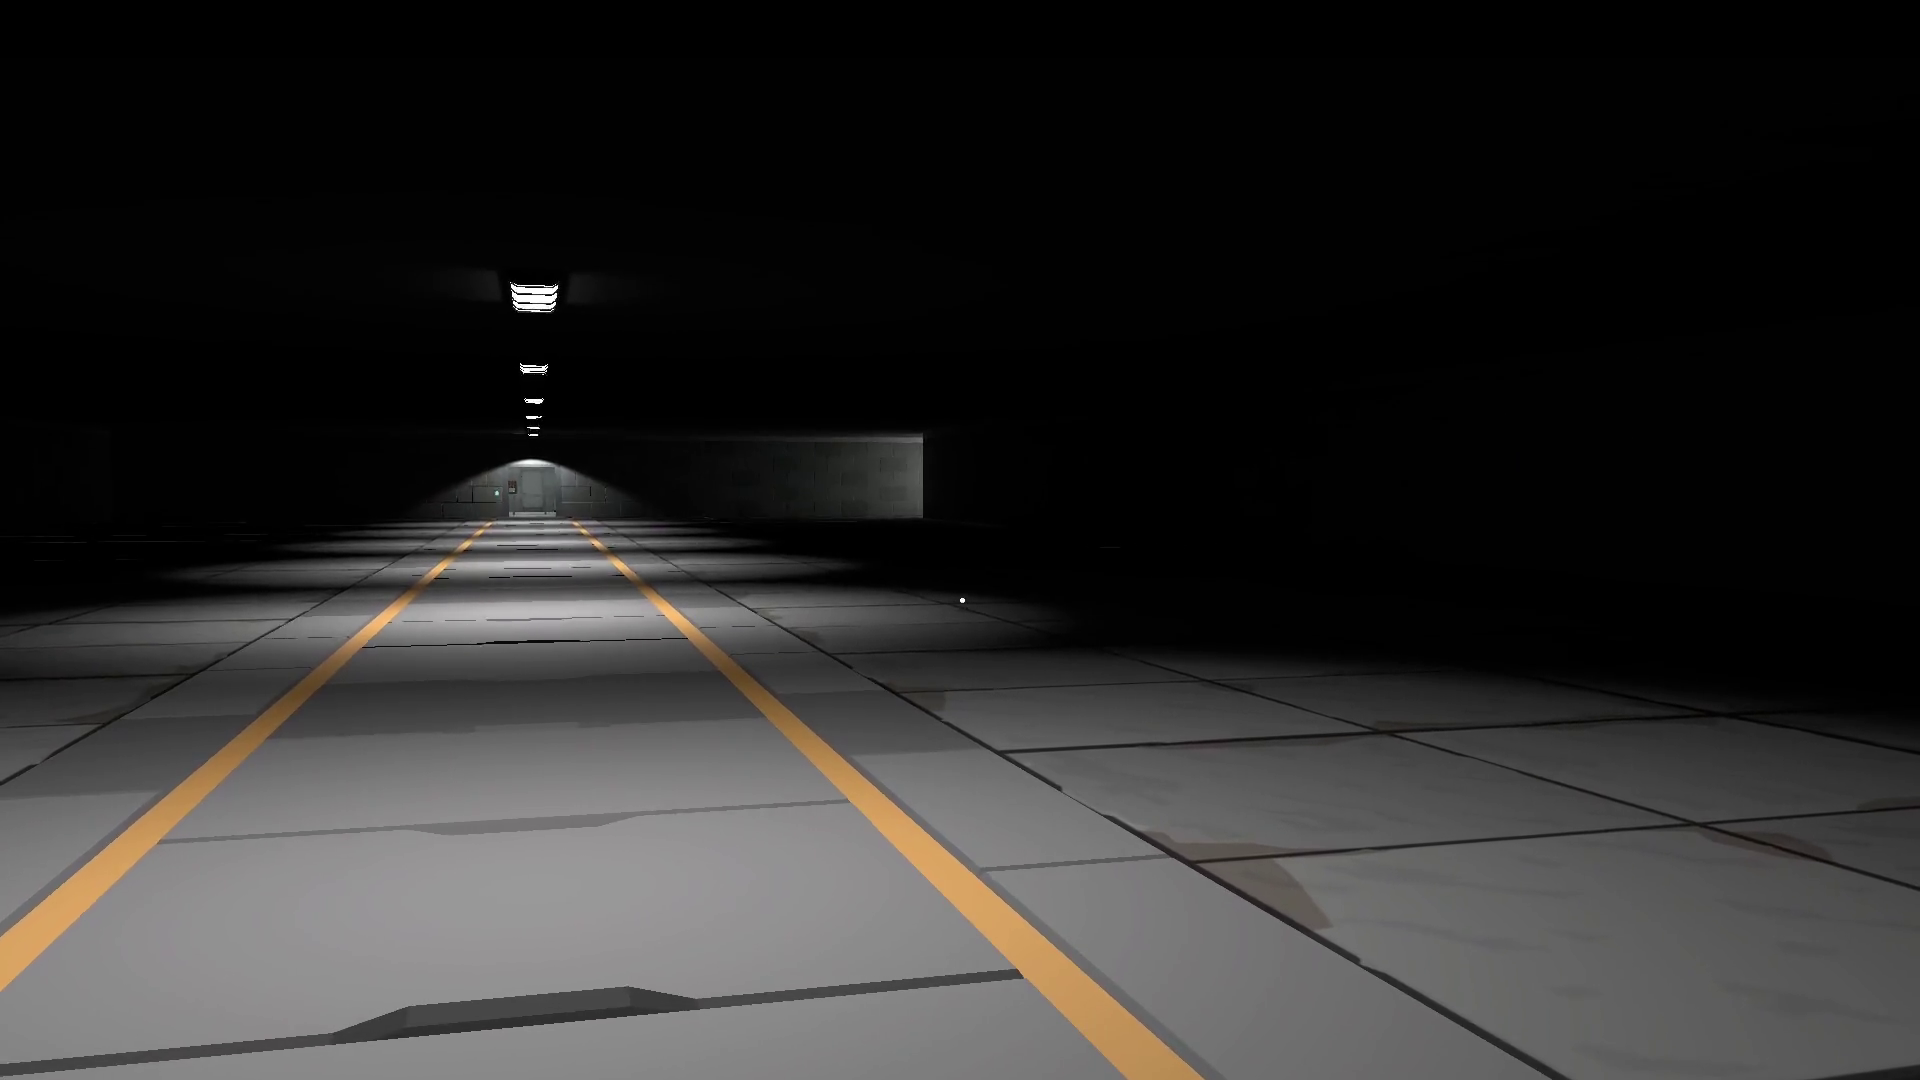}} \\
         \multicolumn{2}{|p{\dimexpr\linewidth-2\tabcolsep}|}{\small \textbf{Figure 7:} Winding Hallway \& Shortcut represented as a partially illuminated room in our game.}\\
        \hline
\end{xtabular}
\vspace{12pt}

\tablefirsthead{}
\tablehead{\hline \multicolumn{2}{|r|} {Continued from previous page} \\ \hline}
\tabletail{\hline \multicolumn{2}{|r|} {Continued on next page} \\ \hline}
\tablelasttail{}

\newpage
\begin{xtabular}{|l|p{\dimexpr\linewidth/2}|}
        \hline
        \multicolumn{2}{|c|}{\textbf{Obstacle Onslaught}} \\
        \hline
        \textbf{Dark Pattern Concept:} & Obstruction \cite{Gray.26.04.2018}\\
        \hline
        \textbf{Strategies:} & FAKE, OBSCURE, VIOLATE \\
        \hline
        \textbf{Related Patterns:} & Aesthetic Manipulation, Nagging, Forced Action, Hidden Information \\
        \hline
        \multicolumn{2}{|l|}{\textbf{Description:}} \\
        \multicolumn{2}{|p{\dimexpr\linewidth-2\tabcolsep}|}
        {The analogy provides players with a seemingly empty room with an immediately visible exit. When they try to get to the exit, a number of obstacles appear to prevent the players from advancing, one after the other. The analogy provides a distraction at each obstacle that promises to advance the players but instead only throws them back. } \\
        \hline
        \multicolumn{2}{|l|}{\textbf{Examples / Known Uses:}} \\
        \multicolumn{2}{|p{\dimexpr\linewidth-2\tabcolsep}|}
        {In our game, the obstacles consist of a simple jump-and-run segment, an invisible labyrinth, a more difficult jump-and-run segment, a series of unnecessary questions, and a search puzzle where players need to find a key. At every obstacle, there is a teleporter that the narrator claims will bring the player to their destination. In actuality, the teleporters do not lead to the destination, but either exhibit strange behavior or lead the players back to a previous teleporter, but never forward.} \\
        \hline
        \multicolumn{2}{|l|}{\textbf{Context:}} \\
        \multicolumn{2}{|p{\dimexpr\linewidth-2\tabcolsep}|}
        {Website providers often employ obstructions to prevent users from performing actions that may improve user privacy. For example, a website may require users in need of support to talk to a chatbot or interactive voice response system before speaking to a human directly. Similarly, a multi-step process may be necessary to delete an account on a website.} \\
        \hline
        \multicolumn{2}{|l|}{\textbf{Effect:}} \\
        \multicolumn{2}{|p{\dimexpr\linewidth-2\tabcolsep}|}
        {Players initially feel like they may easily finish this room by walking through. After each obstacle, it seems like the goal is almost reached but new obstacles keep appearing. The game seems to offer an easier way out but this is only an additional obstacle in the players' way. The only way to get to the exit is by persevering through the obstacles.} \\
        \hline
        \multicolumn{2}{|l|}{\textbf{Countermeasures:}} \\
        \multicolumn{2}{|p{\dimexpr\linewidth-2\tabcolsep}|}
        {Players must resist the temptation of occupying themselves with the distraction and instead persevere through each obstacle to reach their goal. This mirrors real-life examples of Obstruction where users need to persist through barriers or multi-step processes to achieve their objectives rather than quitting the process (thereby failing to achieve their objective) or giving in to an easier way out (such as a special deal offered to users trying to cancel a paid subscription) .} \\
        \hline
        \multicolumn{2}{|l|}{\textbf{Psychological Aspects:}} \\
        \multicolumn{2}{|p{\dimexpr\linewidth-2\tabcolsep}|}
        {Obstruction aims to fatigue players and deter them from getting to the exit. Each obstacle demands System 2 thinking and severe motivation, while quitting or giving in to the distraction would be the System 1 solution, enticing players to take an apparently easier route. After repeated failures with the distraction, players recognize the need to overcome the obstacles for true progress.} \\
        \hline
        \multicolumn{2}{|c|}{\vspace{-7pt}}\\
        \multicolumn{2}{|c|}{\includegraphics[width=\dimexpr\linewidth-2\tabcolsep]{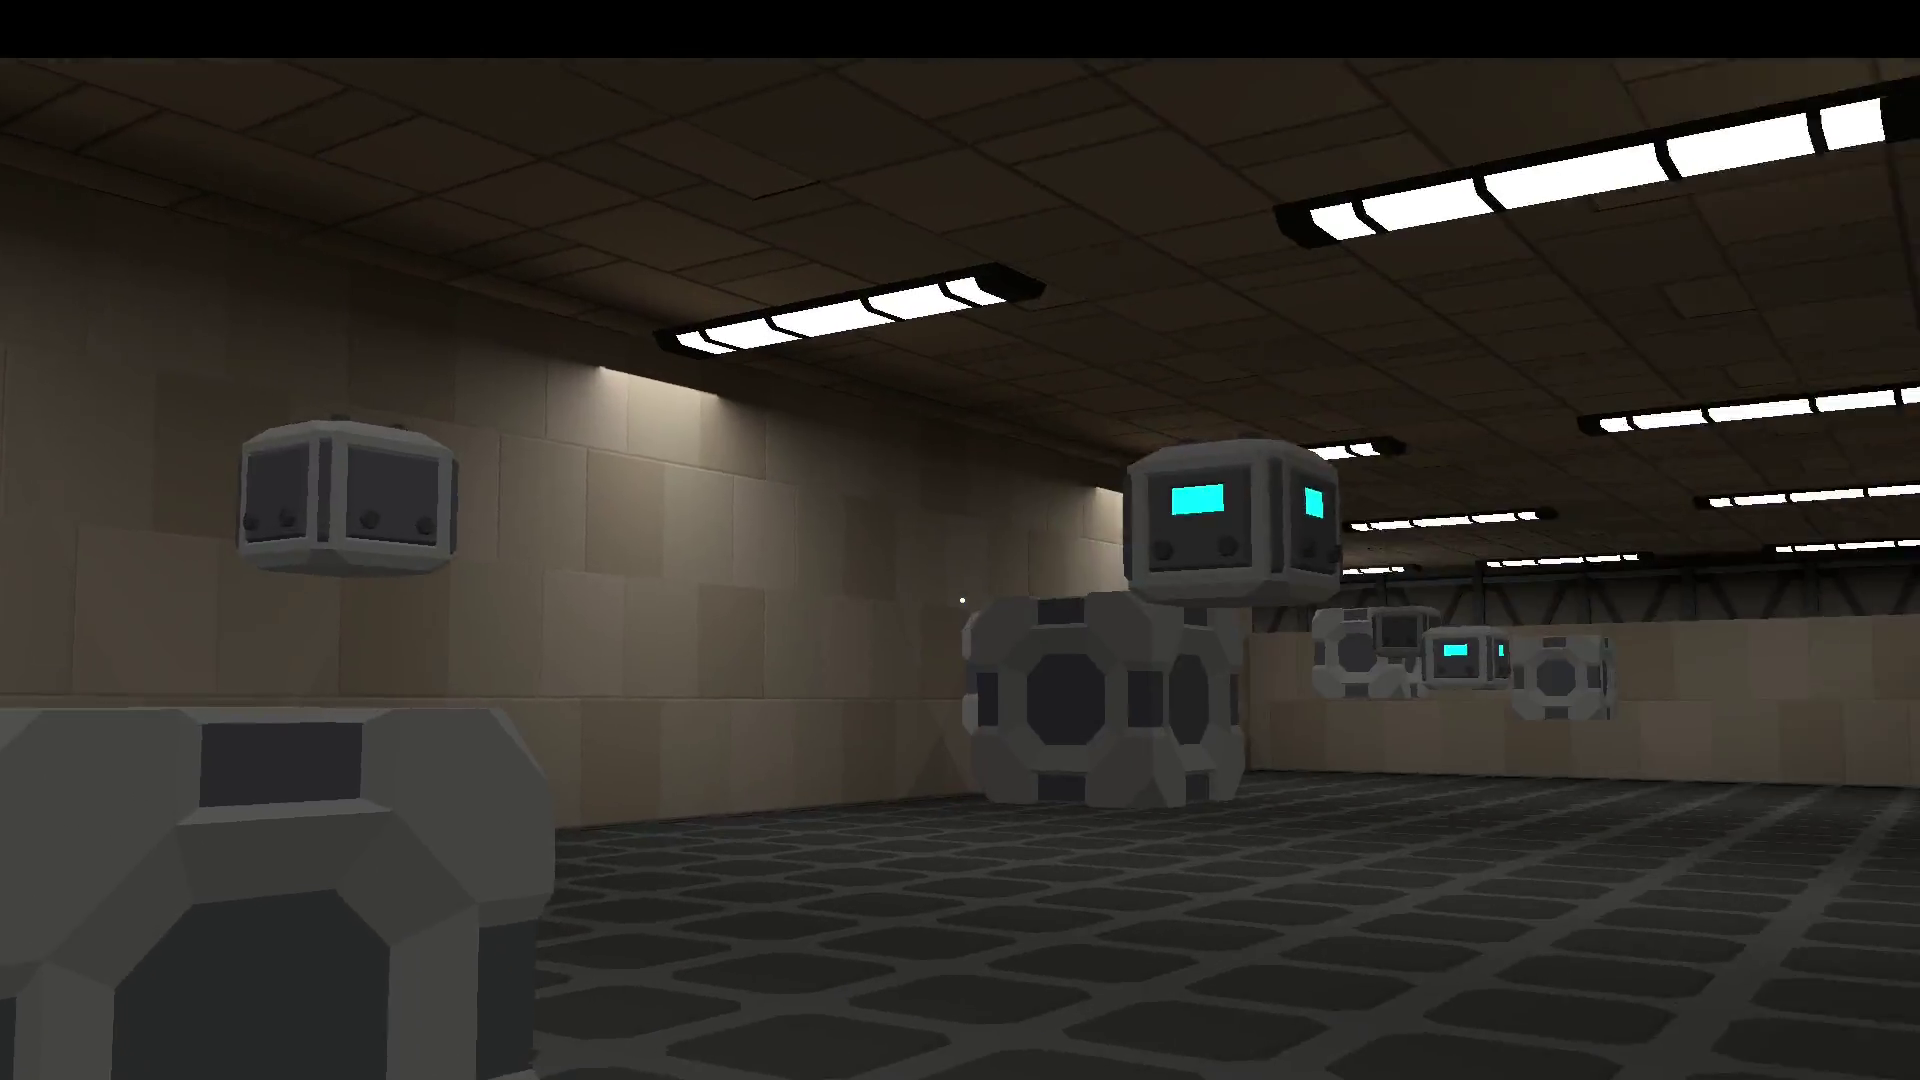}} \\
        \multicolumn{2}{|p{\dimexpr\linewidth-2\tabcolsep}|}{\small \textbf{Figure 8:} Obstacle Onslaught partially represented as a jump-and-run course in our game.}\\
        \hline
\end{xtabular}
\vspace{12pt}

\tablefirsthead{}
\tablehead{\hline \multicolumn{2}{|r|} {Continued from previous page} \\ \hline}
\tabletail{\hline \multicolumn{2}{|r|} {Continued on next page} \\ \hline}
\tablelasttail{}

\begin{xtabular}{|l|l|}
        \hline
        \multicolumn{2}{|c|}{\textbf{Insistent Questioning}} \\
        \hline
        \textbf{Dark Pattern Concept:} & Nagging \cite{Gray.26.04.2018}\\
        \hline
        \textbf{Strategies:} & DENY, MAXIMIZE \\
        \hline
        \textbf{Related Patterns:} & Obstruction, Forced Action \\
        \hline
        \multicolumn{2}{|l|}{\textbf{Description:}} \\
        \multicolumn{2}{|p{\dimexpr\linewidth-2\tabcolsep}|}
        { The analogy gives players a set of objects to bring with them throughout the game. The analogy repeatedly asks the players in various situations to give away the objects to gain a slight advantage. However, while none of the slight advantages are necessary to complete the game, the objects are required to finish a section of the game. Reaching that point without sufficient objects left forces players to backtrack.} \\
        \hline
        \multicolumn{2}{|l|}{\textbf{Examples / Known Uses:}} \\
        \multicolumn{2}{|p{\dimexpr\linewidth-2\tabcolsep}|}
        {At the beginning of the game, the narrator tasks the players with keeping hold of a set of six screws. During each segment of the game, the narrator asks the players to use a screw for various things, such as repairing a squeaking door, a broken monitor, or a teleporter. Before entering the final room of the game, players need to repair a broken number pad using four screws. If they gave too many screws away they need to return to the previous game segment (in this case Obstacle Onslaught) and retrieve a set of screws left there by the narrator.} \\
        \hline
        \multicolumn{2}{|l|}{\textbf{Context:}} \\
        \multicolumn{2}{|p{\dimexpr\linewidth-2\tabcolsep}|}
        {Website and app providers often nag users to gain app permissions or to sell something to them. This is done by repeatedly notifying users of the offer and often only allowing users to either accept or get asked again later, rather than permanently disabling the questions. A prominent example is YouTube Premium advertising that is shown on the mobile app often, as well as Instagram asking for permission to use the location services of the phone.} \\
        \hline
        \multicolumn{2}{|l|}{\textbf{Effect:}} \\
        \multicolumn{2}{|p{\dimexpr\linewidth-2\tabcolsep}|}
        {Players are annoyed by the constant questioning regarding the objects and may get weary as to why they constantly get asked about them. As the game provides no way to stop the questions, the nagging persists and constantly interrupts the flow of gameplay, leading to frustration.} \\
        \hline
        \multicolumn{2}{|l|}{\textbf{Countermeasures:}} \\
        \multicolumn{2}{|p{\dimexpr\linewidth-2\tabcolsep}|}
        {Players need to ignore the requests to avoid the negative consequence of having to backtrack to gain more objects. This is akin to app users being unable to stop the constant nagging from the app and having to always dismiss the nagging notification to preserve their privacy.} \\
        \hline
        \multicolumn{2}{|l|}{\textbf{Psychological Aspects:}} \\
        \multicolumn{2}{|p{\dimexpr\linewidth-2\tabcolsep}|}
        {This educational dark pattern analogy exploits players' psychological susceptibility to System 1 thinking by consistently pressuring them to relinquish crucial objects for small short-term gains. Unlike real examples of Nagging, where the negative consequences are only ever apparent long after the manipulation by the dark pattern, the consequence of giving away too many objects is made apparent to the players within the game session.} \\
        \hline
        \multicolumn{2}{|c|}{\vspace{-7pt}}\\
        \multicolumn{2}{|c|}{\includegraphics[width=\dimexpr\linewidth-2\tabcolsep]{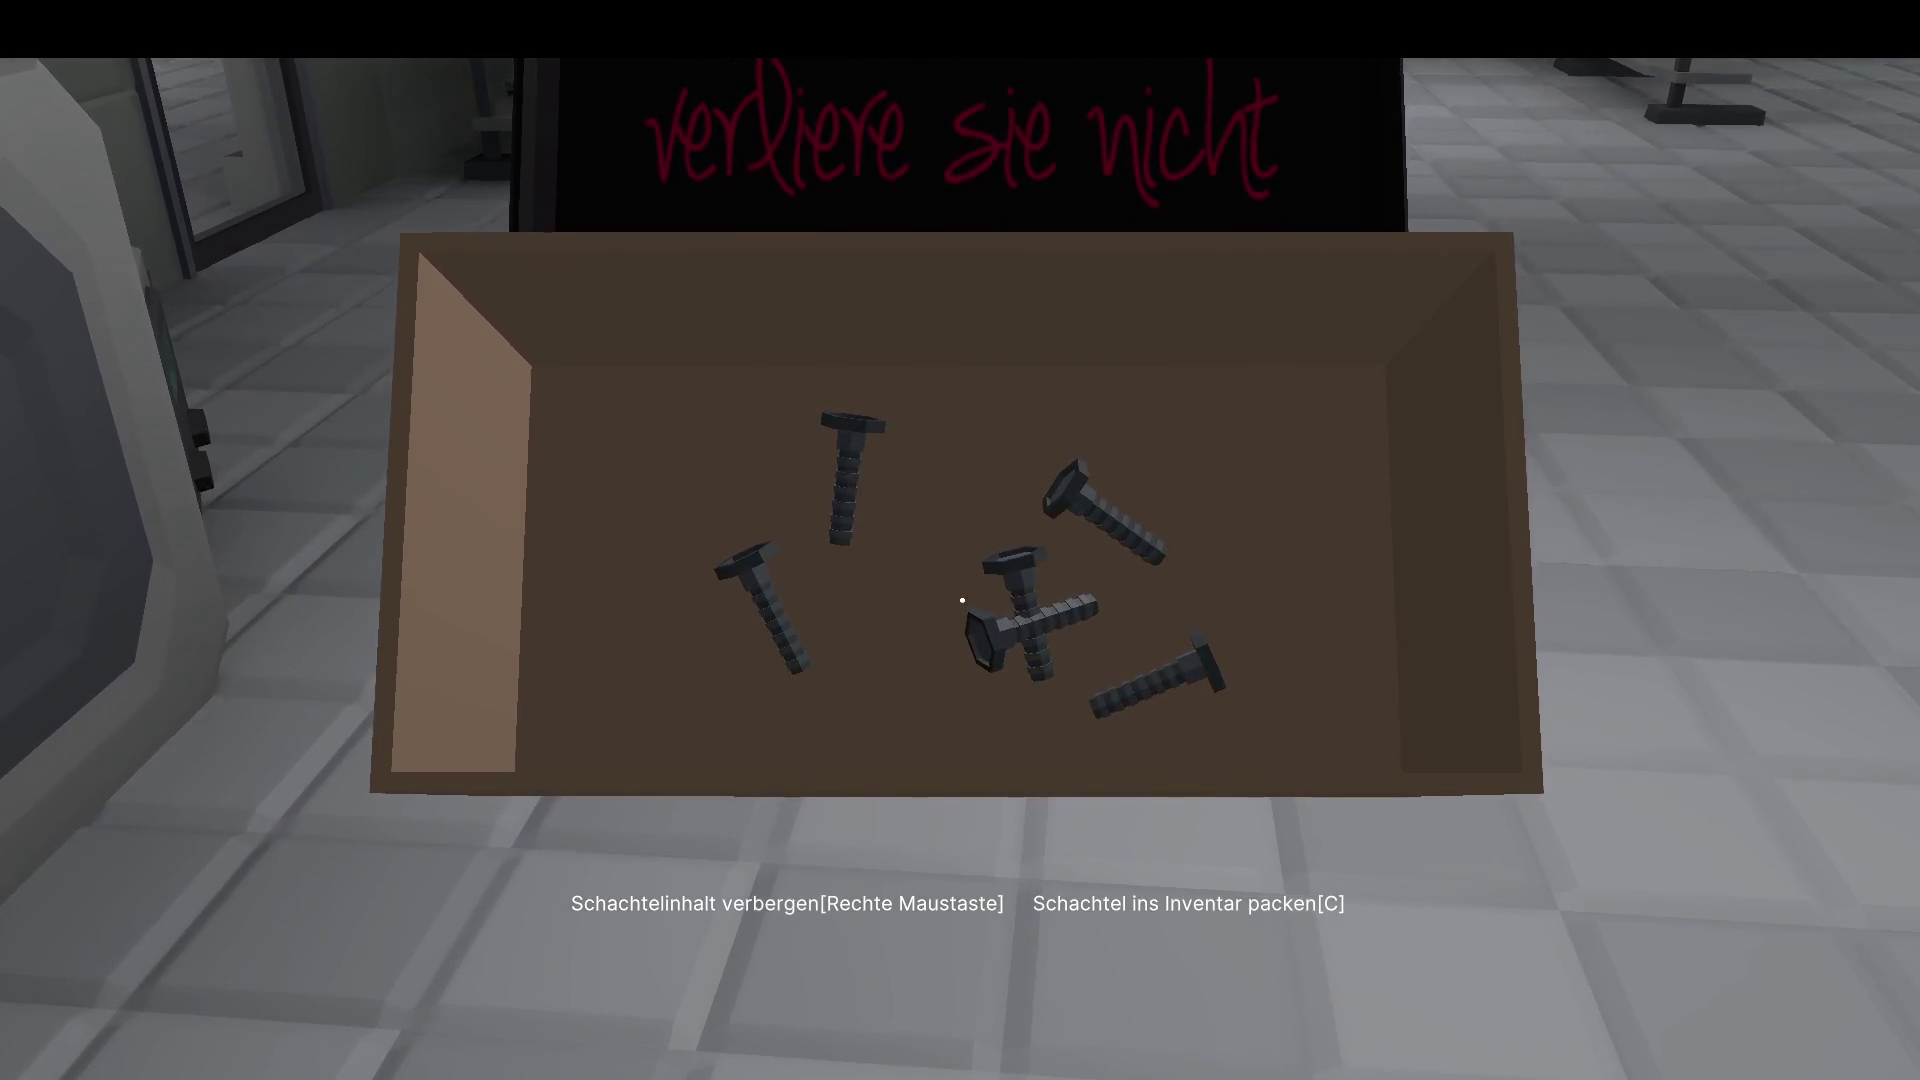}} \\
        \multicolumn{2}{|p{\dimexpr\linewidth-2\tabcolsep}|}{\small \textbf{Figure 9:} Insistent Questioning represented by a set of screws in our game.}\\
        \hline
\end{xtabular}
\vspace{12pt}

\tablefirsthead{}
\tablehead{\hline \multicolumn{2}{|r|} {Continued from previous page} \\ \hline}

\tabletail{\hline \multicolumn{2}{|r|} {Continued on next page} \\ \hline}
\tablelasttail{}

\begin{xtabular}{|l|p{\dimexpr\linewidth/2}|}
        \hline
        \multicolumn{2}{|c|}{\textbf{Looping Gameplay}} \\
        \hline
        \textbf{Dark Pattern Concept:} & Forced Action \cite{Gray.26.04.2018}\\
        \hline
        \textbf{Strategies:} & DENY, MAXIMIZE \\
        \hline
        \textbf{Related Patterns:} & Obstruction, Nagging \\
        \hline
        \multicolumn{2}{|l|}{\textbf{Description:}} \\
        \multicolumn{2}{|p{\dimexpr\linewidth-2\tabcolsep}|}
        {The analogy lets players encounter a situation in the game that prompts them to repeat a large section of the game to proceed once they return. The analogy provides a plausible reason for this, however, players can never fulfill the requirements necessary to proceed beyond this point. The only option is to leave the game, which the analogy provides hints at.} \\
        \hline
        \multicolumn{2}{|l|}{\textbf{Examples / Known Uses:}} \\
        \multicolumn{2}{|p{\dimexpr\linewidth-2\tabcolsep}|}
        {In our game, players find themselves in a room that has a door labeled “Exit”. When trying to open it, the narrator reveals that the players were part of an experiment and have not yet collected enough data for the experiment to be completed. A teleporter emerges from the ground which players can use to return to the start of the game. After completing the Insensible Key Mapping scenario again, they are returned to the Looping Gameplay room, as if having completed the game again, visualized by a fade-to-black. This repeats indefinitely while hand-written hints appear on the walls prompting the players to close the game.} \\
        \multicolumn{2}{|l|}{\textbf{Context:}} \\
        \multicolumn{2}{|p{\dimexpr\linewidth-2\tabcolsep}|}
        {Some websites only allow users to use their services if they first perform an action seemingly unrelated to the service provided. Examples include forced consent for data collection on news platforms and forced registration for mortgage calculations. Users have the choice to either perform the forced action or disengage from the service without finishing their task.} \\
        \hline
        \multicolumn{2}{|l|}{\textbf{Effect:}} \\
        \multicolumn{2}{|p{\dimexpr\linewidth-2\tabcolsep}|}
        {The lack of an apparent alternative drives players to replay the section of the game that needs to be repeated. The repetitions increase player frustration and should ideally stay in the players' minds even after playing the game, ideally reemerging when they are forced to do something they do not want to do to access a service.} \\
        \hline
        \multicolumn{2}{|l|}{\textbf{Countermeasures:}} \\
        \multicolumn{2}{|p{\dimexpr\linewidth-2\tabcolsep}|}
        {The only available countermeasure against Forced Action is refraining from using the service in the first place. Similarly, the only available countermeasure to repeating the game is to quit playing the game entirely.} \\
        \hline
        \multicolumn{2}{|l|}{\textbf{Psychological Aspects:}} \\
        \multicolumn{2}{|p{\dimexpr\linewidth-2\tabcolsep}|}
        {This educational dark pattern analogy plays on the psychological concept of sunk cost and the fear of missing out. By presenting players with a plausible reason to repeat a large section, the game fosters a belief in an achievable goal. However, the deliberate impossibility of fulfilling the requirements creates a sense of frustration and entrapment. Players grapple with the emotional investment made versus the rational choice to disengage. Unlike in real examples of Forced Action however, the game eventually provides hints to the fact that they can and should quit, teaching the players the necessary countermeasure to avoid the Forced Action dark pattern.} \\
        %\hline
        \multicolumn{2}{|c|}{\vspace{-7pt}}\\
        \multicolumn{2}{|c|}{\includegraphics[width=\dimexpr\linewidth-2\tabcolsep]{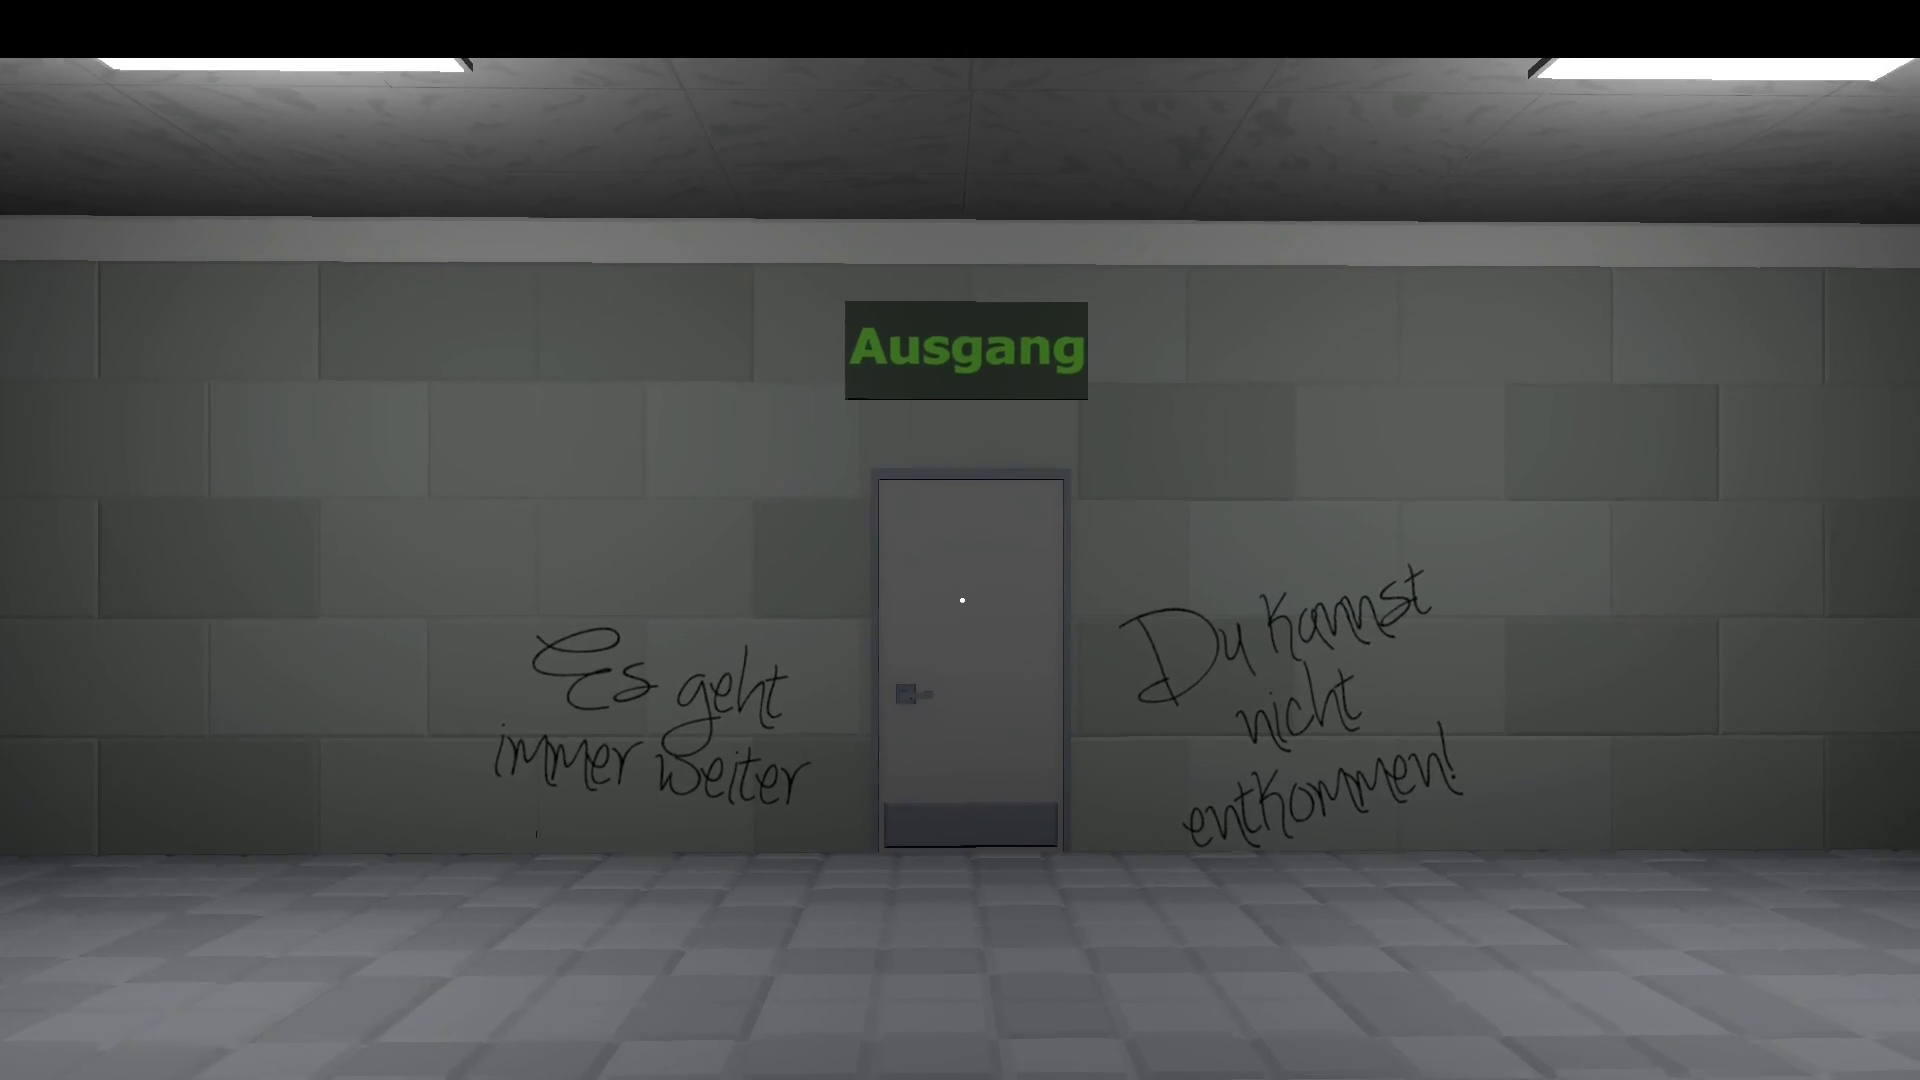}} \\
        \multicolumn{2}{|p{\dimexpr\linewidth-2\tabcolsep}|}{\small \textbf{Figure 10:} Looping Gameplay represented as a permanently closed Exit in our game.}\\
        \hline
\end{xtabular}
%\vspace{-12pt}

\newpage
\section{Appendix B: Scripts and Descriptions from the Online Survey Study}
Our online survey study used commentated videos of each educational dark pattern analogy. This appendix provides English versions of the scripts for these videos and the corresponding definitions of dark pattern concepts used in the online survey study.

\subsection{Introduction}

Thank you for participating in our study.

In this study, we are investigating dark patterns - manipulative interaction techniques that are used by website/app operators to get you to behave in a certain way that is not in your best interest. Website/app operators do that by taking advantage of certain psychological behavioral patterns of people to influence their behavior. 

To better inform people about dark patterns and their effects, we have developed an educational video game. In it, you play a new employee in a laboratory. Your boss, the lab manager, uses manipulative tricks to get you to spend as much time in the lab as possible. Each room in the game represents a dark pattern. In this study, you will see commented excerpts from this video game and then compare them with descriptions and explanations of dark patterns.

\subsection{Insensible Key Mapping / Preselection}
This room is about familiarizing yourself with the controls of the game. The lab manager asks you whether you want to use a "preferred control" selected by him. If you accept the "preferred control", you realize that this "preferred control" does not follow any known pattern and is difficult to understand. The lab manager explains that you can customize the controls in the menu.
 
"Preselection" is a dark pattern where an option is preselected before you interact with a website or app. The operators want this option to be retained, although this option is often not in your interest and could have unintended consequences for you.

\subsection{Sneaky Shop / Sneaking}
The laboratory manager shows you the Shoppifier 3000. You are supposed to use this machine to produce items from a list that you need for your work in the laboratory. In the next step, these items are sent for disinfection, where only exactly the items on the list are accepted. 

If you now believe that you have selected exactly the items that are on the list in the Shoppifier, it can still happen that your selection is rejected during disinfection. The reason is that the Shoppifier has - unbeknownst to you - selected additional items that it considered matching.

"Sneaking" is a dark pattern in which website/app operators try to hide or disguise information that is relevant to you or only reveal it with delay. The aim is to get you to do something that you would not have done if the information had not been hidden.

\subsection{Walls of Text / Hidden Information}
You enter a room with four screens. On those screens, you see long texts. There are also eight large control levers on the floor. The lab manager tells you to read the texts in order to learn the rules of the lab. To prove that you have read the texts carefully, you must move the switches to the correct alignment. In each text there is a hidden reference to a button. If you press it, a puzzle will appear for you to solve. Once this has been solved, you will be shown part of the correct switch combination. Once you have read all four screens and solved the corresponding puzzles, you will know the complete switch combination.

"Hidden Information" is a dark pattern in which website/app operators try to hide certain information or make it difficult to access by displaying it on the website. This can be options that are hidden behind an interaction, or important information that is hidden in small or discolored text. The aim is to disguise important information as unimportant information.

\subsection{Winding Hallway \& Shortcut / Aesthetic Manipulation}
You enter a large room that is only illuminated in the middle. The lab manager asks you to follow the illuminated path. When you reach the center of the room, you hear a noise from the darkness on the left. The lab manager asks you to ignore it and continue on. If you follow the illuminated path, you will come to a long, winding hallway with advertising posters, to which the lab manager will read out advertising messages until you reach the next room after a long walk. If you follow the noise to the side of the room into the darkness instead, you will find a hidden door under a broken lamp that leads to a dark but short hallway to the next room. Finally, both possible hallways lead to the next room.

"Aesthetic Manipulation" is a dark pattern that is more concerned with presentation than content. Website/app operators present several equivalent options in significantly different ways so that your attention is drawn to the options that benefit the operator more and distract you from options that would benefit you more.

\subsection{Obstacle Onslaught / Obstruction}
You arrive in an initially empty room that you have to cross - which seems easy. However, when you try to cross it, the floor lowers and several floating blocks appear, which you have to jump over to get to the other side. A teleporter will also appear which, according to the lab manager, can teleport you directly to the end of the room. However, none of the buttons on the teleporter seem to work, only the color of the teleporter changes. If you cross the floating blocks, a wall and an invisible labyrinth appear, as well as a second teleporter, which teleports you to the beginning instead of the end of the room, namely to the first teleporter. If you find a way through the invisible labyrinth instead, new floating blocks and another teleporter will appear, which only rotates around itself. If you jump over the floating blocks across the wall, a bridge will appear which you can only cross if you answer the questions of the lab manager. However, if you reach the door at the end of the room, it will not open. The teleporter next to the door will only take you back to the previous teleporters. You can only open the door by finding a hidden key.   

"Obstruction" is a dark pattern in which website/app operators make a task more difficult for you than it would be on its own. This is intended to prevent you from completing the task. For example, certain tasks that you want to achieve may be blocked by large obstacles.

\subsection{Insistent Questioning / Nagging}
At the beginning of the game, the lab manager gives you a box of screws with the task of carrying them with you and not losing them. In each room of the game, the lab manager will ask you to use a screw to repair something. This is not necessary to progress in the game - but the lab manager asks you in a way that doesn't make that clear. Towards the end of the game, however, you will need four screws to repair a broken combination lock. If you have given away too many screws beforehand, you have to run back and get new screws. 

"Nagging" is a dark pattern where website/app operators repeatedly interrupt your experience on the website/app to get you to behave in a certain way that is not directly related to what you are trying to achieve.

\subsection{Looping Gameplay / Forced Action}
You enter a room with a door with a sign above it saying "Exit". However, when you try to open the door, it does not open. The lab manager explains that your stay in the lab was an experiment and that you have not yet collected enough data for him. He says that you can pass through the exit when you have collected enough data. You can now return to the start of the game via a teleporter to comply with this request. The game then starts again from the beginning. When you reach the exit again, the lab manager repeats that you have not collected enough data and sends you back to the start of the game. Each time you reach the exit, a new message will appear on the wall telling you that the lab manager will not let you leave. The only way out is to end the game via the menu.

"Forced Action" is a dark pattern in which website/app operators require you to do something additional in order to achieve your actual goal - otherwise you cannot reach it.
